# Supplementary material for: InstaFace: Identity-Preserving Facial Editing with Single Image Inference
Source: arXiv:2502.20577 source file (2025-03-07)
Supplement: Supplementary file 1 [file X_suppl.tex]

\clearpage
\setcounter{page}{1}
\maketitlesupplementary

\section{Visualization of the Impact of Facial \mbox{Recognizer}}

This section provides further analysis and visualizations to demonstrate the qualitative impact of the Facial Recognizer (FR) on maintaining identity-specific features in our model. As mentioned in Section 5.3, the difference in re-identification accuracy (Re-ID) with and without FR may seem minor in Table~\ref{tab:facial_recognizer_ablation}. However, this does not fully capture the FR's qualitative impact on preserving key identity features. In Figure~\ref{fig:ablationfr}, row 1 illustrates the result from the model without the facial recognizer (Base + CLIP, abbreviated as B+C). Here, the resultant identity deviates from the original image, which is, in this case, Joe Biden, leading to differences in features like the eyes, nose, and mouth. When comparing the model with (Base + CLIP + Facial Recognizer, abbreviated as B+C+F) and without the FR, we can observe improvements in preserving key features, especially the eye positioning—where the distance between the eyes appears more natural in B+C+F. Additionally, the lower teeth are more accurately represented according to the pose when using B+C+F, which is a notable difference compared to B+C. Furthermore, in row 2 of Figure~\ref{fig:ablationfr}, the model that utilizes the FR shows a more natural appearance in the cheek region, highlighting the importance of the FR in refining minor facial details that contribute to the realistic perception of identity. While the quantitative improvements are small, visual comparisons demonstrate that the Facial Recognizer is essential in preserving identity by refining key regions such as the eyes, nose, mouth, and overall facial structure.

\begin{figure}[!h]
    \centering
    \includegraphics[width=\linewidth]{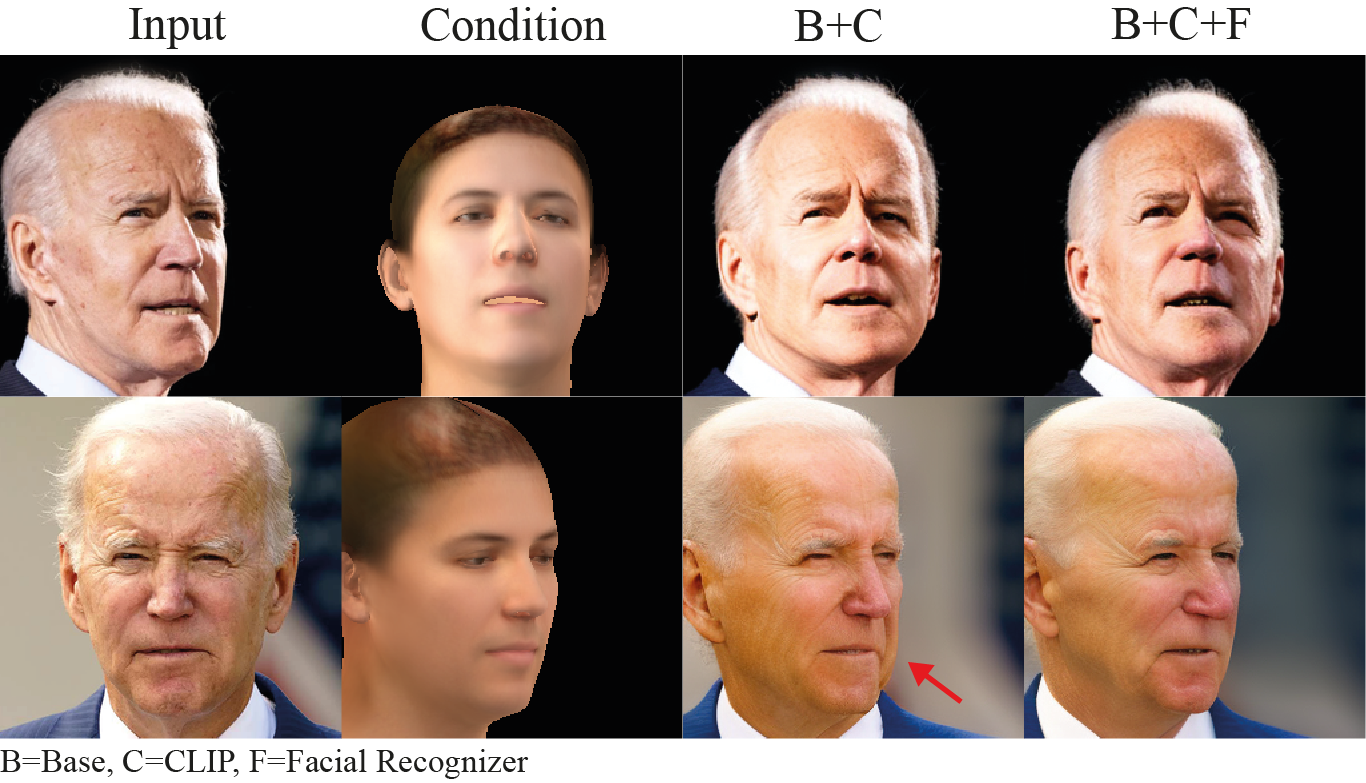} % Include your image here
    \caption{In row 1, the absence of the Facial Recognizer (B+C) leads to deviations in facial features, such as a narrower eye distance and missing lower teeth. In row 2, artifacts are present in the cheek region without the Facial Recognizer. Including the FR (B+C+F) corrects these issues, leading to better identity retention.}
    
    % In row 1, differences in facial shape, mouth, nose, and eyes between B+C and B+C+F are observed, significantly impacting overall identity preservation. In row 2, the cheek region in B+C appears as an artifact due to improper editing, whereas B+C+F effectively corrects these details, resulting in better identity retention. These observations highlight the crucial role of the Facial Recognizer in maintaining consistent facial identity.

    \label{fig:ablationfr}
\end{figure}

\section{Discussion on Single Image Inference}

\subsection{Contribution of Diffusion Network Blocks}

The objective of this experiment is to evaluate the impact of different blocks in our model during the process of single-image fine-tuning. Generally, during fine-tuning, the Guidance Network remains inactive, and the entire Diffusion Network is trained. However, in this experiment, we freeze most of the Diffusion Network and focus on training only one block of interest, such as Downblock, Midblock, or Upblock. This allows us to observe and analyze the individual contribution of each block. As shown in Figure ~\ref{fig:block_ablation}, the Downblock primarily captures coarse facial features but fails to retain the identity and background details like hair and hands. The Midblock exhibits similar limitations. In contrast, the Upblock effectively preserves identity and background features, highlighting its crucial role in fine-tuning. Since the UpBlock is the most effective, we also evaluate to determine which module (residual, self-attention, or cross-attention) within the UpBlock contributes most significantly during fine-tuning.
% The Downblock, depicted in Figure ~\ref{fig:block_ablation}, mainly captures the fundamental structural components, such as the background and large edges, ensuring they are preserved. The Midblock, however, faces challenges in preserving its distinctiveness or providing comprehensive information about its origins. In contrast, the Upblock successfully preserves the image's background and identity, emphasizing its importance in fine-tuning. 

\vspace{0.2cm}
\begin{figure}[ht]
    \centering
    \includegraphics[width=\linewidth]{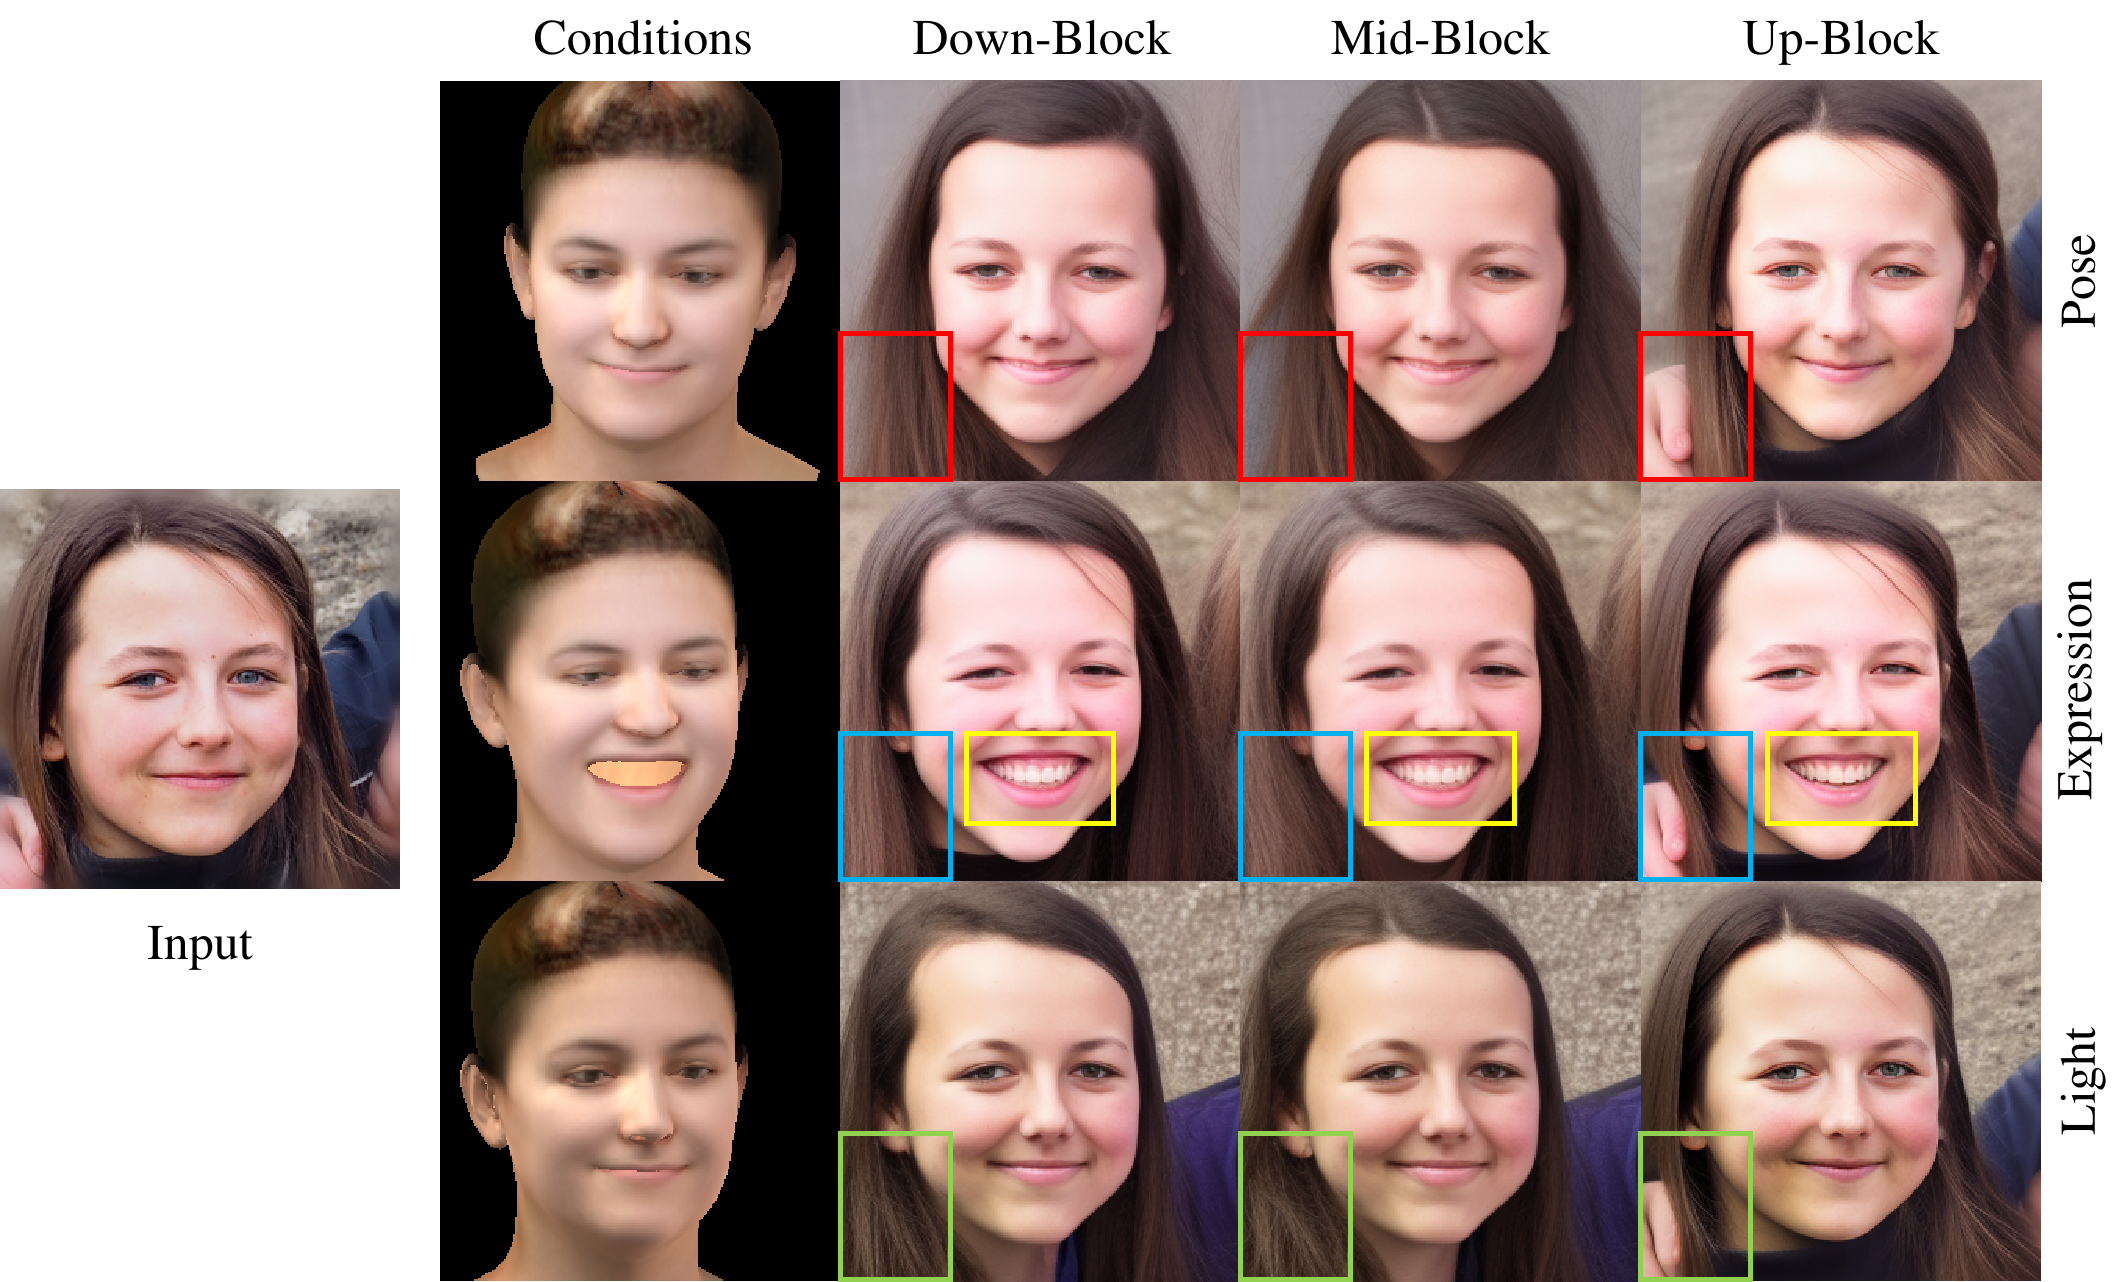} % Include your image here
    \vspace{0.1cm}
    \caption{Impact of different blocks of Diffusion Network during single-image fine-tuning. Only the Upblock (right column) effectively preserves the image's background and identity. The rectangles represent the area of observation.}
    \label{fig:block_ablation}
\end{figure}

\subsection{Effectiveness of Modules in the UpBlock}
Unlike traditional methods like IP-Adapter~\cite{ye2023ip}, I2V-Adapter~\cite{guo2023i2v}, and Stable Diffusion, which utilizes and modifies cross-attention mechanisms for the required semantic alignment with the input, our experiments during single-image fine-tuning reveal a different dynamic. Figure \ref{fig: ablation} shows that the ResNet layers in the upsampling block are primarily updated, which is crucial for retaining input-output similarity, including background, hair, and accessories. In this study, we train only the layers shown in each row of Figure \ref{fig: ablation}, freezing all other layers to identify which updates best preserve identity and background details.

\vspace{0.4cm}
\begin{figure}[!h]
    \centering
    \includegraphics[width=\linewidth]{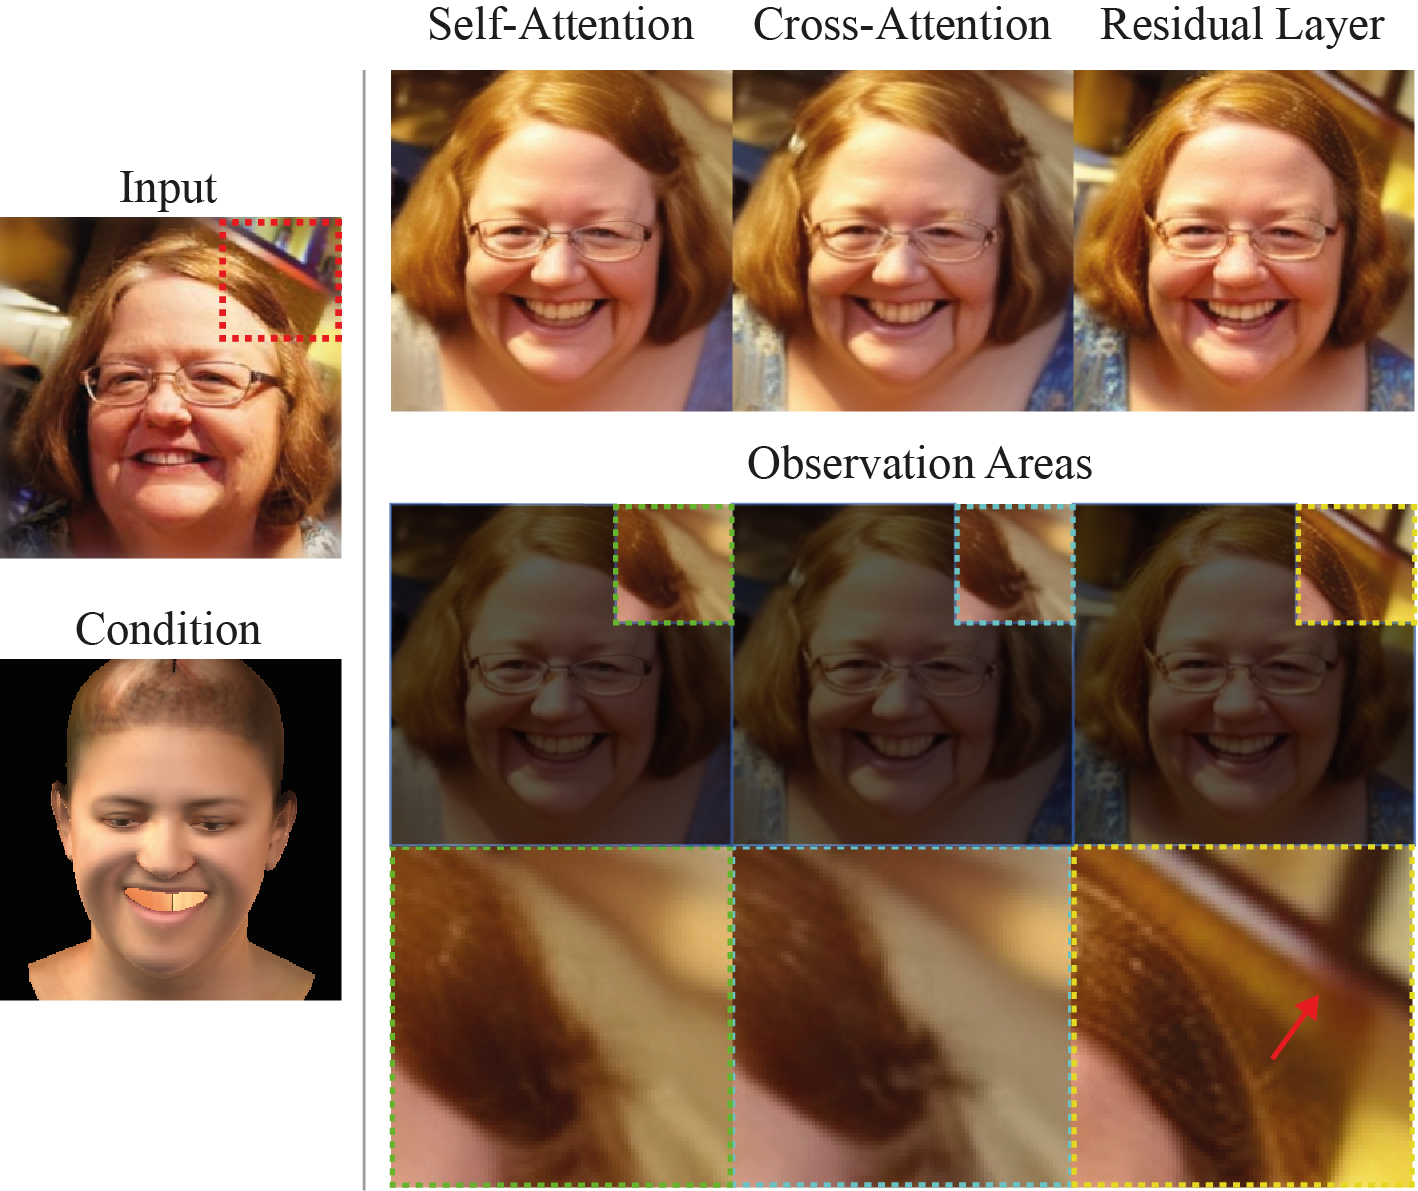} % Include your image here
    \caption{Impact of residual, self-attention, and cross-attention layers from the upsample block during single-image fine-tuning. The results highlight that residual layers are instrumental in preserving both background elements and critical facial features, ensuring consistency in the generated image. The squares and arrow symbols indicate areas of interest for observing these effects.}
    \label{fig: ablation}
\end{figure}

\section{Architecture Details}

In this section, we provide details of our model's architecture and training. We employ Stable Diffusion 1.4 (SD 1.4) as the base generative model \cite{rombach2022high}, and the RetinaFace\cite{deng2019retinaface} model is used as the facial recognizer. The projection module in our model includes perceiver attention\cite{jaegle2021perceiver} layers and feed-forward components, transforming embeddings into latent representations for cross-attention. Detailed hyperparameters and architectural configurations are summarized in Table~\ref{tab:architectural_training_details}.

\begin{table}[!htbp]
\centering
\caption{Architectural and Training Details of Our Model}
\setlength{\tabcolsep}{6pt} % Reduced column spacing for better readability
 % Increased row height for more vertical space
\small % Reduce font size for the table content
\resizebox{\columnwidth}{!}{ % Resize the table to fit the column width
\begin{tabular}{l l}
    \toprule
    \textbf{Parameter} & \textbf{Value} \\
    \midrule
    \multicolumn{2}{l}{\textbf{Model Information}} \\
    \vspace{2pt} % Add vertical space between sections
    \hspace{5mm}Base Model & Stable Diffusion 1.4 (SD 1.4) \\
    \hspace{5mm}Facial Recognizer & RetinaFace \\ 
    \hspace{5mm}Image Input Size & 256 $\times$ 256 \\

    \midrule
    \multicolumn{2}{l}{\textbf{Training Hyperparameters}} \\
    \vspace{2pt} % Add vertical space between sections
    \hspace{5mm}Learning Rate & $1.0 \times 10^{-5}$ \\
    \hspace{5mm}Adam Beta1 & 0.9 \\
    \hspace{5mm}Adam Beta2 & 0.999 \\
    \hspace{5mm}Adam Weight Decay & $1.0 \times 10^{-2}$ \\
    \hspace{5mm}Adam Epsilon & $1.0 \times 10^{-8}$ \\
    \hspace{5mm}Num Training Timesteps & 1000 \\
    \hspace{5mm}Beta Start & 0.00085 \\
    \hspace{5mm}Beta End & 0.012 \\
    \hspace{5mm}Beta Schedule & Scaled Linear \\
    \hspace{5mm}Noise Offset & 0.05 \\
    \hspace{5mm}SNR Gamma & 5.0 \\

    \midrule
    \multicolumn{2}{l}{\textbf{Architectural Configuration}} \\
    \vspace{2pt} % Add vertical space between sections
    \hspace{5mm}Activation Function & SiLU \\
    \hspace{5mm}Attention Head Dimension & 8 \\
    \hspace{5mm}Sample Size & 64 \\
    \hspace{5mm}Input Channels & 4 \\
    \hspace{5mm}Output Channels & 4 \\
    \hspace{5mm}Block Output Channels & [320, 640, 1280, 1280] \\
    \hspace{5mm}Projection Module Depth & 4 \\
    \hspace{5mm}Projection Module Heads & 20 \\
    \hspace{5mm}Projection Module Queries & 16 \\
    \hspace{5mm}Projection Module Output Dimension & 1280 \\
    
    \bottomrule
\end{tabular}}
\label{tab:architectural_training_details}
\end{table}

\vspace{0.5cm}
\begin{figure}[!ht]
    \centering
    \includegraphics[width=\columnwidth]{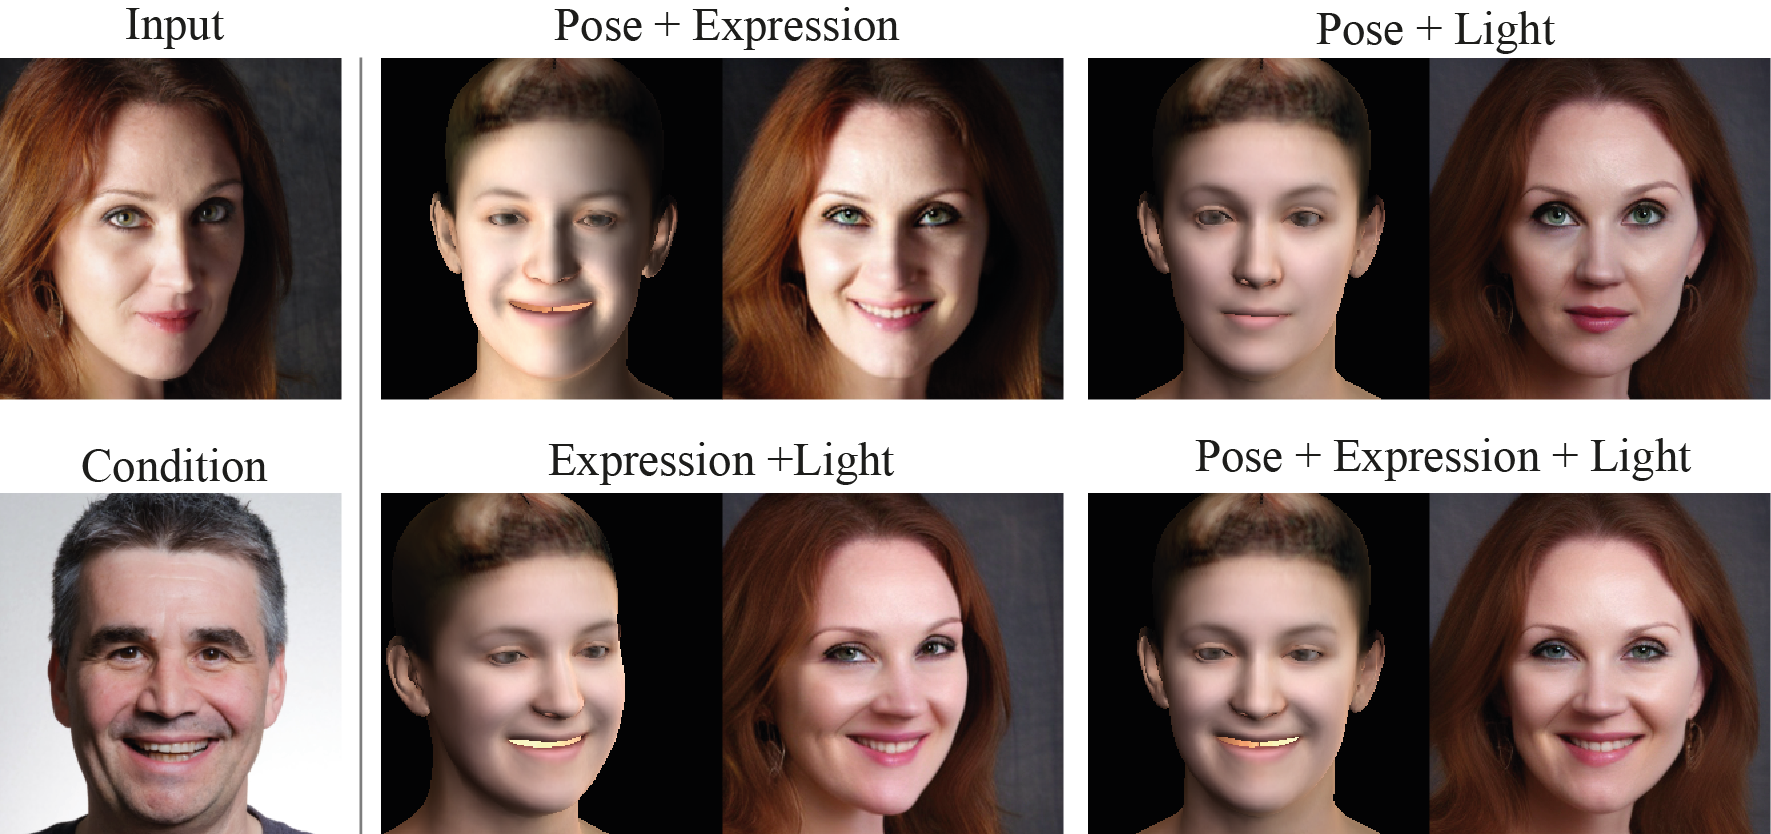} % Update with your figure path
    \vspace{0.1cm}
    \caption{Visualization of Attribute Editing Combinations. Each pair illustrates different combinations of attribute editing, \eg pose + expression, pose + lighting. The left image in each pair represents the corresponding conditional maps for the required edit, while the right image shows the generated output.}
    \label{fig:combo}
\end{figure}

\section{Supplementary Examples}
In this section, we present additional examples to demonstrate the effectiveness of our method in manipulating facial attributes. Figure~\ref{fig:combo} illustrates different combinations of attribute editing, such as pose + expression and pose + lighting, showcasing the flexibility of our approach. Subsequently, Figure~\ref{fig:more_examples} provides a detailed example of individual attribute transfer. Here, pose, expression and lighting conditionals are extracted from a target image and applied to an input image. The results demonstrate that our method effectively transfers these attributes while preserving the input's identity and other vital features.

\begin{figure*}[h]
    \centering
    \includegraphics[width=0.95\textwidth]{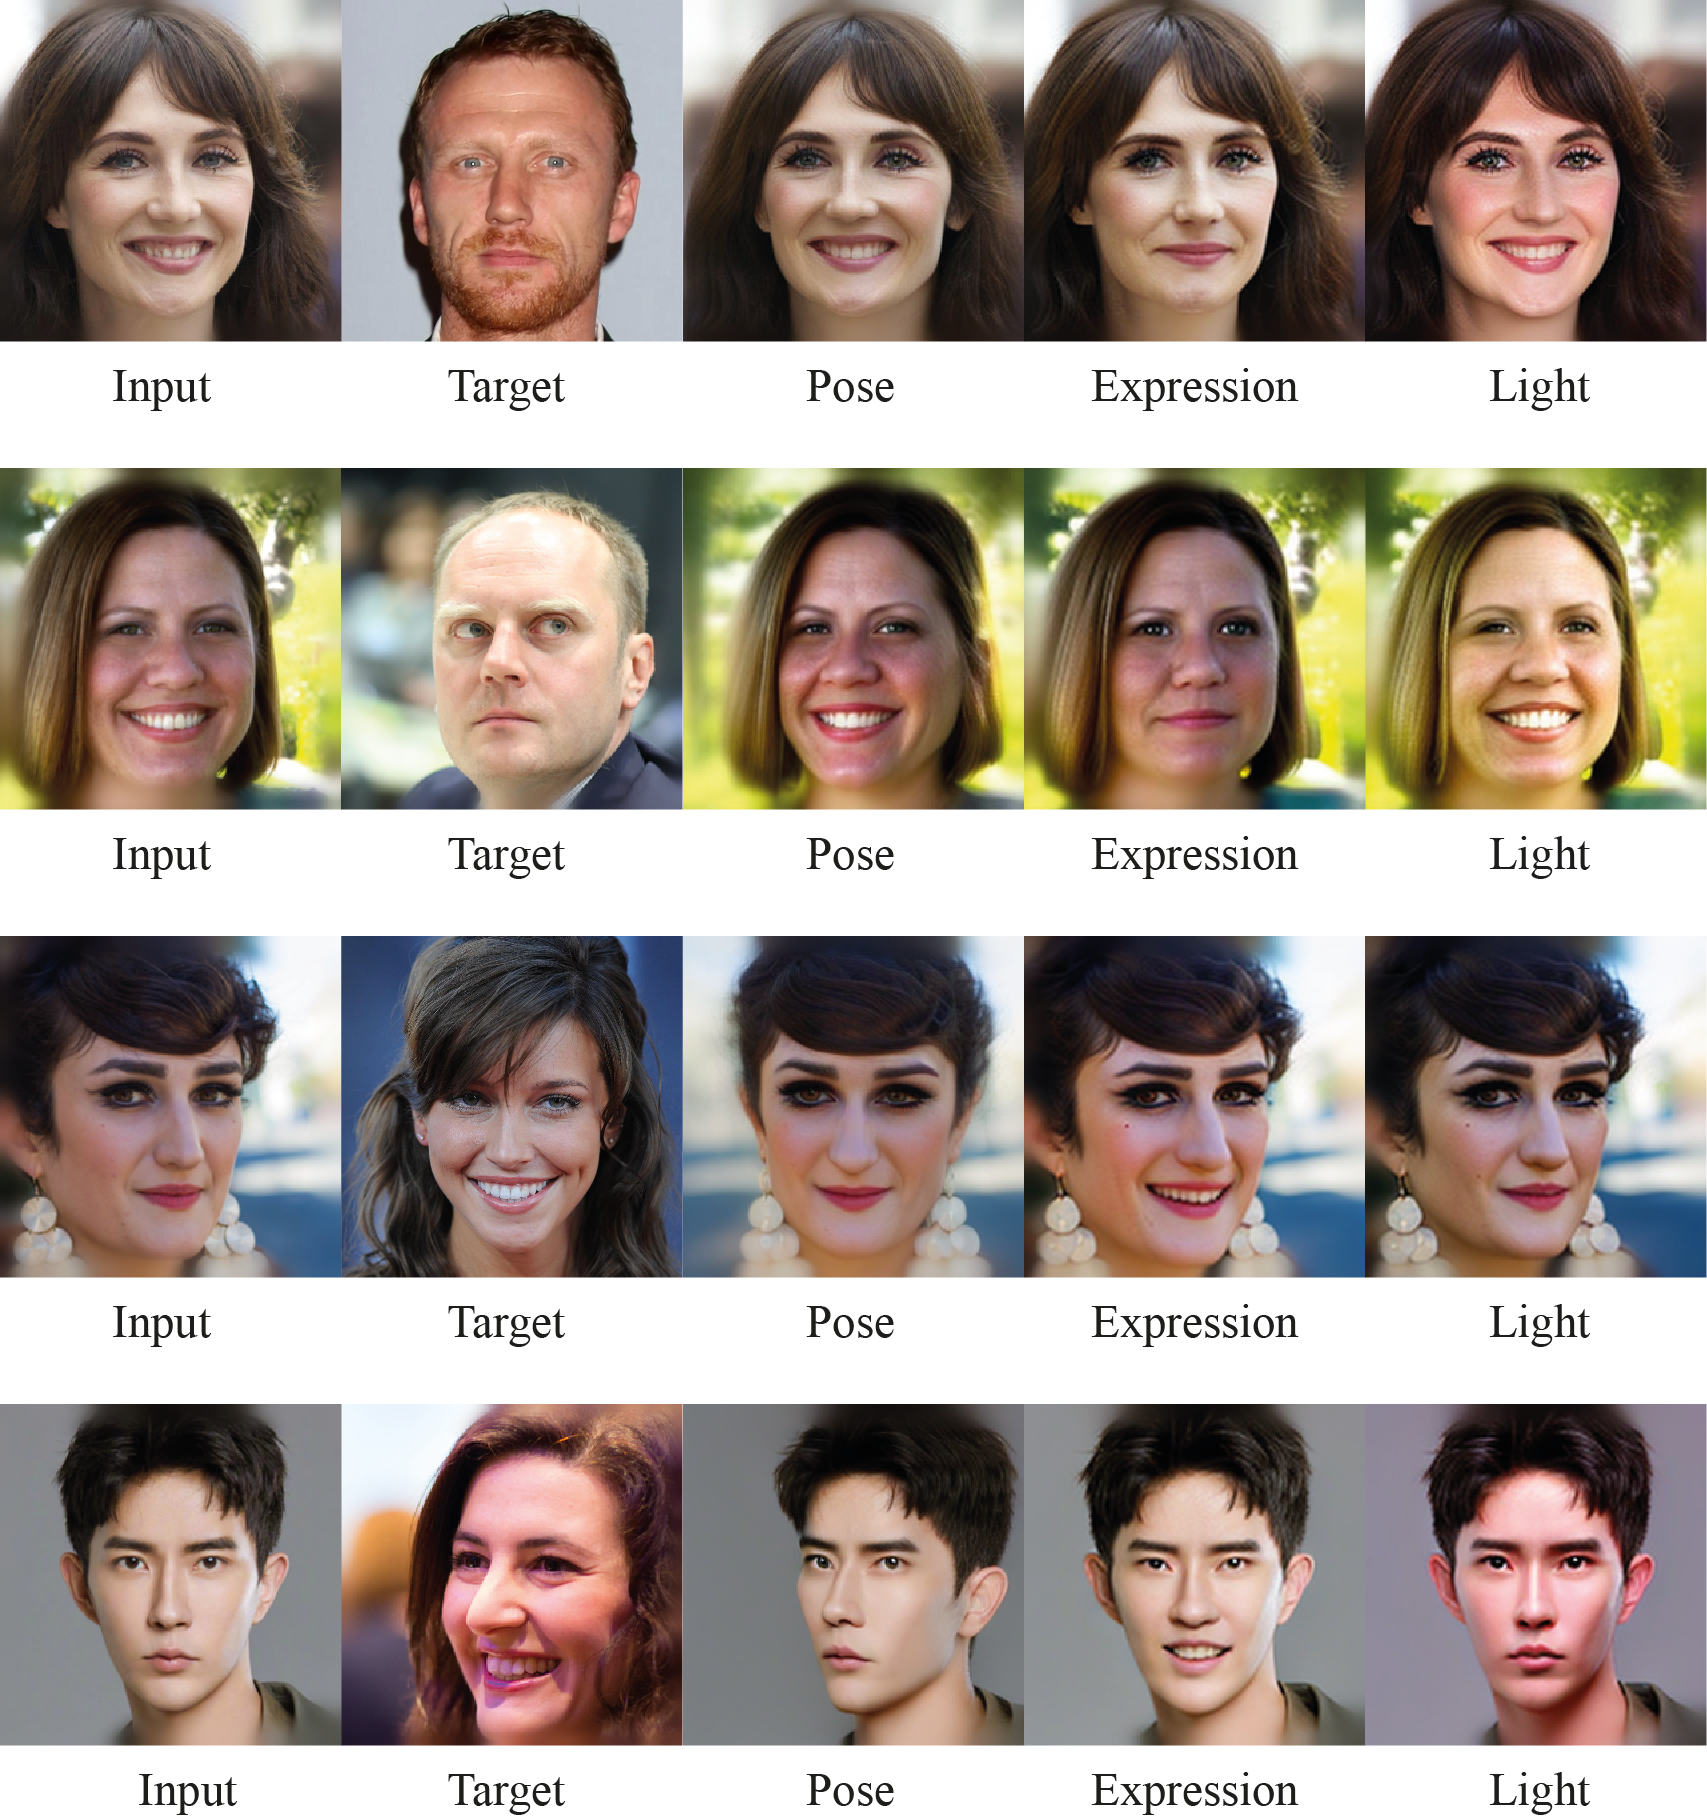}
    \caption{Examples of facial attribute transfer. The conditionals (pose, expression, and lighting) are extracted from various target images and applied to corresponding input images. The results demonstrate the successful transfer of these attributes while maintaining the identity and key features of the input images across different instances.}
    \label{fig:more_examples}
\end{figure*}

% In this section, we provide additional examples to illustrate the efficacy of our methodology in manipulating facial attributes. We employ an image of Barack Obama as the driving or target image, as illustrated in Figure ~\ref{fig:more_examples}. The attributes of the image, including pose, expression, and lighting, are replicated. The provided input images to the model depict Joe Biden. The results illustrate how our method successfully transfers the target attributes from the Barack Obama image to the Joe Biden image while preserving the input's identity and other significant features.
